# Supplementary material for: DocFormerv2: Local Features for Document Understanding
Source: arXiv:2306.01733 source file (2023-06-02)
Supplement: Supplementary file 1 [file appendix.tex]

\section{Supplemental}

%You must include your signed IEEE copyright release form when you submit your finished paper. We MUST have this form before your paper can be published in the proceedings.

This is the supplemental material for the main DocFormer paper \cite{appalaraju2021docformer}. Please read the main paper for model formulation, performance numbers on various datasets and further analysis and ablation. 

\subsection{Implementation Details} We present all the hyper-parameters in Table \ref{table:implementation_full_1} used for pre-training and fine-tuning \papertitle. We fine-tune on downstream tasks on the same number of epochs as prior art \cite{xu2020layoutlm,xu2020layoutlmv2,bros2020hong}: FUNSD \cite{jaume2019}, Kleister-NDA \cite{gralinski2020kleister} datasets were fine-tuned for 100 epochs. CORD \cite{park2019cord} for 200 epochs. RVL-CDIP \cite{harley2015icdar} for 30 epochs. For Key, Query 1-D relative local attention we choose a span of $8$ i.e. for a particular multi-modal feature, \papertitle gives more attention $8$ tokens to its left and right.

\begin{table}[H]
	\begin{center}
	\scalebox{0.85}{
		\begin{tabular}{l|c|c}
			Hyper-Parameter & Pre-training & Fine-tuning \\
			\Xhline{2.5\arrayrulewidth}
			Epochs & 5 & varies \\
			Learning rate & 5E-05 & 2.5E-05 \\
			Warm-up & 10\% iters & 0 \\
			Gradient Clipping & 1.0 & 1.0 \\
			Gradient agg. & False & False \\
			Optimizer & AdamW\cite{loshchilov2017decoupled} & AdamW\cite{loshchilov2017decoupled} \\
			Lower case & True & True  \\
			Sequence length & 512 & 512 \\
			Encoder layers & 12 & 12 \\
			32-bit mixed precision & True & True \\
			Batch size & 9 per GPU & 4 per GPU \\
			GPU hardware & A100 (40GB) & V100 (16GB) \\
			Training Num. Samples & 5M & varies \\
			Training time & 17 hours/epoch & varies \\
			%\hline
			%%\Xhline{2.5\arrayrulewidth}
		\end{tabular}
		}
	\end{center}
	\vspace{-3ex}
	\caption{\textbf{Implementation Details}: Hyper-parameters used for pre-training \papertitle and fine-tuning for downstream tasks. Training epochs vary for down-stream tasks.}
	\label{table:implementation_full_1}
	\vspace{-1ex}
\end{table}

\subsection{Run-time Complexity Analysis}
Since we propose a variant of the self-attention \cite{vaswani2017attention} operation, we compute the train and inference run-time analysis in big-o notation.

\begin{table}[H]
	\begin{center}
	\scalebox{0.85}{
		\begin{tabular}{l|c|c}
			Layer Type & Run-time Complexity & Seq. Complexity \\
			\Xhline{2.5\arrayrulewidth}
			Convolution & $O\left(k \cdot n \cdot d^{2}\right)$ & $O(1)$  \\
			Recurrent & $O\left(n \cdot d^{2}\right)$ & $O(n)$ \\
			Self-Attention & $O\left(n^{2} \cdot d\right)$ & $O(1)$ \\
			Self-Attention (relative) & $O\left(r \cdot n \cdot d\right)$ & $O(1)$ \\
			\papertitle MMSA & $2 \cdot [ O\left(n^{2} \cdot d\right) ]$ & $O(1)$ \\
		\end{tabular}
		}
	\end{center}
	\vspace{-3ex}
	\caption{\textbf{Complexity analysis}: Here $n$ is the sequence length, $d$ is the representation dimension, $k$ is the kernel
size of convolutions and $r$ the size of the neighborhood in restricted self-attention. Omitting number of attention heads $h$ for brevity. Here assume $h=1$. In addition, MMSA: multi-modal self-attention.}
	\label{table:implementation_full}
	\vspace{-1ex}
\end{table}

Please note that the full run-time complexity for \papertitle has been abridged as the self-attention is the most significant operation (keeping in line with big-O notation). In addition, the presence of $2$ is to signify the unique MMSA operation proposed in this paper, where multi-modal feature from each layer is added with image and spatial features (see Section 3.1). We see that DocFormer's multi-modal self-attention (Section 3.1) is an efficient way to do multi-modal learning.

\subsection{Pseudo-code}
We present a rough pseudo-code for our novel multi-modal self-attention (MMSA) as described in section 3.1. We believe the pseudo-code would aid an independent researcher to better replicate our proposed novelty. Please note omitting dropout and layer norm at the end for brevity.

\begin{lstlisting}[language=Python]
##Multi Modal Self Attention

#text kqv embeddings
key1 = Linear(d_model, n_head * d_k)
query1 = Linear(d_model, n_head * d_k)
value1 = Linear(d_model, n_head * d_v)

#image kqv embeddings
key2 = Linear(d_model, n_head * d_k)
query2 = Linear(d_model, n_head * d_k)
value2 = Linear(d_model, n_head * d_v)

#spatial embeddings. note! shared by text, image
key3 = Linear(d_model, n_head * d_k)
query3 = Linear(d_model, n_head * d_k)

#See Eq. 6 and 7 in main paper for formulation
def multi_modal_self_attention(emb, img_feat, spatial_feat):

  #self-attention of text (and prev. layers subseq.)
  k1,q1,v1 = emb,emb,emb
  k1 = rearr(key1(k1), 'b t (head k) -> head b t k')
  q1 = rearr(query1(q1), 'b l (head k) -> head b l k')
  v1 = rearr(value1(v1), 'b t (head v) -> head b t v')
  attn1 = einsum('hblk,hbtk->hblt', [q1,k1])/sqrt(q1.shape[-1])

  #1D relative pos. (query, key)
  #note rel_pos_embed1 is learnt relative pos emb. nxn
  rel_pos_key1 = einsum('bhrd,lrd->bhlr', k1, rel_pos_embed1)
  rel_pos_query1 = einsum('bhld,lrd->bhlr', q1, rel_pos_embed1)

  #shared spatial - text/hidden features
  sp_k1, sp_q1 = spatial_feat, spatial_feat
  sp_k1=rearr(key3(sp_k1),'b t (head k) -> head b t k')
  sp_q1=rearr(query3(sp_q1),'b l (head k)->head b l k')
  text_only_spatial_scores = einsum('hblk,hbtk->hblt', [sp_q1,sp_k1])/sqrt(sp_q1.shape[-1])

  text_attn_scores = attn1 + rel_pos_key1 + rel_pos_query1 + text_only_spatial_scores

  #-----
  ##Self-attn of image (repeat of above for img feat)
  k2,q2,v2 = img_feat,img_feat,img_feat
  k2 = rearr(key2(k2), 'b t (head k) -> head b t k')
  q2 = rearr(query2(q2), 'b l (head k) -> head b l k')
  v2 = rearr(value2(v2), 'b t (head v) -> head b t v')
  attn2 = einsum('hblk,hbtk->hblt', [q2,k2])/sqrt(q2.shape[-1])

  #1D relative pos. (query, key)
  #note rel_pos_embed1 is learnt relative pos emb. nxn
  rel_pos_key2 = einsum('bhrd,lrd->bhlr', k2, rel_pos_embed2)
  rel_pos_query2 = einsum('bhld,lrd->bhlr', q2, rel_pos_embed2)

  #shared spatial - img features
  sp_k2, sp_q2 = spatial_feat, spatial_feat
  sp_k2=rearr(key3(sp_k2),'b t (head k) -> head b t k')
  sp_q2=rearr(query3(sp_q2),'b l (head k)->head b l k')
  img_only_spatial_scores = einsum('hblk,hbtk->hblt', [sp_q2,sp_k2])/sqrt(sp_q2.shape[-1])

  img_attn_scores = attn2 + rel_pos_key2 + rel_pos_query2 + img_only_spatial_scores

  #---- attended output: multi-modal
  text_attn_probs = dropout(softmax(dim=-1)(text_attn_scores))
  img_attn_probs = dropout(softmax(dim=-1)(img_attn_scores))
  
  text_cntx = einsum('hblt,hbtv->hblv', [text_attn_probs, v1])
  img_cntx = einsum('hblt,hbtv->hblv', [img_attn_probs, v2])
  context = text_cntx + img_cntx
  return context
\end{lstlisting}

\subsection{\papertitle Architecture for Downstream Tasks}
\papertitle is pre-trained as mentioned in section 3.2. After training it for 5 epochs, we remove the pre-training multi-task heads and use \papertitle (including the visual branch) as a backbone. We simply add a trainable linear-head which predicts the appropriate number of classes which is dataset specific. 
Please see Figure \ref{fig:downstream_arch} for architecture modifications for downstream tasks.

\begin{figure*}[hbt!]
	\centering
	\subcaptionbox{Architecture for downstream Document Classification Task}[.45\linewidth][c]{%
	\includegraphics[width=\linewidth]{images/DocFormer_finetune_global.pdf}}\quad
	\subcaptionbox{Architecture for downstream Sequence and Entity Labeling Tasks}[.45\linewidth][c]{%
	\includegraphics[width=\linewidth]{images/DocFormer_finetune_token.pdf}}\quad
	\caption{\textbf{\papertitle architecture for various downstream tasks}: Image on \textbf{Left} (a) is the architecture for document classification [CLS] is a pooling layer (fn $\shortrightarrow$ ReLU $\shortrightarrow$ fn) to get a pooled representation used for document classification task. Image on \textbf{Right} (b) is the architecture used for entity and sequence labeling tasks. Note, only a single linear layer is added for all downstream tasks. Also, all components of \papertitle are fine-tuned for each of the downstream tasks.}
	\label{fig:downstream_arch}
\end{figure*}

\subsection{\papertitle Multi-Modal Self-Attention} In Figure \ref{fig:mm_self_attn_supp} we show a more detailed visual representation of the novel multi-modal self-attention introduced in this paper.  For reference we also show the original self-attention used by Vaswani et al. \cite{vaswani2017attention}.
\begin{figure*}[hbt!]
\begin{center}
%\fbox{\rule{0pt}{2in} \rule{.9\linewidth}{0pt}}
\includegraphics[width=1.0\linewidth]{images/self_atten.pdf}
\end{center}
   \caption{\textbf{Multi-Modal Self-Attention Layer}: the image \textbf{a) Left} shows the traditional self-attention proposed in Vaswani et al \cite{vaswani2017attention}. Note the multi-head attention and feed-forward layers are omitted for brevity. Cross (X) is matrix-multiplication and (+) is element-wise addition. \textbf{b) Right} shows the proposed multi-modal self-attention layer. This comprises each layer of \papertitle. Notice, the spatial weights across text, vision are shared (RED color), thus helping \papertitle address the \textit{cross-modality feature correlation} issue commonly faced in multi-modal training. The notation is consistent with Equations 1-7 in the main paper. Best viewed in color.}
\label{fig:mm_self_attn_supp}
\end{figure*}

\subsection{FUNSD Vizualizations}
\papertitle achieves state-of-the-art performance of 83.34\% F1-score (see Section 4.1) on FUNSD \cite{jaume2019} dataset amongst other multi-modal models its size. In this sub-section we look at more visualizations by \papertitle on the test-set. One important aspect of this VDU we would like to mention is the OCR is not in human reading-order.

Please note that, we search for and present cases where mistakes were made by \papertitle with the aim of understanding mistakes. Legend for the colors used in images is, Header-label: \textcolor{red}{\textbf{Red}}, Question: \textcolor{blue}{\textbf{Blue}}, Answer: \textcolor{green}{\textbf{Green}}, Other: Grey color. Please see Figures \ref{fig:funsd_supplemental_viz3}, \ref{fig:funsd_supplemental_viz1}, \ref{fig:funsd_supplemental_viz2}.

In Figure \ref{fig:funsd_supplemental_atten_map}, we show one specific pattern that \papertitle learns through its novel multi-modal self-attention. We show that \papertitle automatically learns repetitive local patterns even though it was not explicitly taught this.

\begin{figure*}
	\centering
    \subcaptionbox{Ground Truth}[.47\linewidth][c]{%
	\includegraphics[width=\linewidth]{images/FUNSD_best_viz_gt_82837252.png}}\quad
	\subcaptionbox{\papertitle predictions}[.47\linewidth][c]{%
	\includegraphics[width=\linewidth]{images/FUNSD_best_viz_pred_82837252.png}}\quad

	\caption{\textbf{\papertitle perfect predictions for 82837252 testfile of FUNSD dataset}: Left image shows GT and right image is the prediction made by \papertitle which perfectly matches with GT. Best viewed in color.} 

	\label{fig:funsd_supplemental_viz3}
\end{figure*}

\begin{figure*}[hbt!]
	\centering
	\subcaptionbox{Ground Truth}[.47\linewidth][c]{%
	\includegraphics[width=\linewidth]{images/82250337_0338_viz_gt.png}}\quad
	\subcaptionbox{\papertitle predictions}[.47\linewidth][c]{%
	\includegraphics[width=\linewidth]{images/82250337_0338_viz_pred_GREAT.png}}\quad
	\caption{\textbf{\papertitle slightly bad predictions for 82250337\_0338 test\-file on FUNSD dataset}: Based on the predictions on the right (b), we can see that \papertitle was able to classify most of the sequence correctly. However, if we look at the orange bounding boxes we can spot the errors. "(Indicate Distributor's Cost per Carton)" is tagged as Other text in ground-truth but \papertitle incorrectly classified part of the tokens as \textcolor{blue}{\textbf{Question}}. Best if viewed digitally and in color.}
	\label{fig:funsd_supplemental_viz1}
\end{figure*}

\begin{figure*}
	\centering
	\subcaptionbox{Ground Truth}[.47\linewidth][c]{%
	\includegraphics[width=\linewidth]{images/FUNSD_error_viz_gt_87528380.png}}\quad
	\subcaptionbox{\papertitle predictions}[.47\linewidth][c]{%
	\includegraphics[width=\linewidth]{images/FUNSD_error_viz_pred_87528380.png}}\quad
	\caption{\textbf{\papertitle slightly bad predictions for 87528380 testfile on FUNSD dataset}: Here, we focus the readers attention on two specific scenarios: FUNSD dataset has been known to have ground-truth annotation issues. We  find on the left image the orange highlighted box $"8650"$ is incorrectly annotated in GT as $"other"$ text, however \papertitle correctly predicts it as "answer" token for the question $"total"$. \textbf{Scenario 2:} The orange highlighted boxes on the right image are tokens which are actually sub-headers but \papertitle mis-classifies as $"question"$ tokens. In this case, \papertitle likely gave more weight-age to language features and not so much to visual features and so ended up mis-classifying. We would like to point out that this is an ambiguous example as the language in mis-classified regions do look like $"questions"$. Best viewed in color. }
	\label{fig:funsd_supplemental_viz2}
\end{figure*}

\begin{figure*}
	\centering
    \subcaptionbox{Example FUNSD document with Ground Truth overlays}[.40\linewidth][c]{%
	\includegraphics[width=\linewidth]{images/docformer_funsd_attention_example.png}}\quad
	\subcaptionbox{\papertitle prediction self-attention heatmap (last encoder layer, 2nd head). DocFormer has up to 512 tokens in each layer. Each point on the image shows the strength of attention from a token on the $y$-axis to a token on the $x$-axis. The bluer colors show more attention and the red less attention.
	}[.40\linewidth][c]{%
	\includegraphics[width=\linewidth]{images/docformer_funsd_attention.png}}\quad

	\caption{\textbf{\papertitle learns repetition and regularity}: the \textcolor{yellow}{\textbf{yellow}} and \textcolor{magenta}{\textbf{purple}} boxes in the left figure matches the  \textcolor{yellow}{\textbf{yellow}} and \textcolor{magenta}{\textbf{purple}} boxes in the right figure. The OCR is not in reading order. Hence the six occurrences of ``DIVISION" appear together in front (among the top 25) - \textcolor{yellow}{\textbf{yellow}} box in Figure b) and they correspond to the \textcolor{yellow}{\textbf{yellow}} boxes in Figure a).
	Similarly, the \textcolor{magenta}{\textbf{purple}} box in Figure b) corresponds to the \textcolor{magenta}{\textbf{purple}} boxes in Figure a).
	\papertitle is able to pick up such repetitions as strong self-attention signals (blue colored pixels in the right self-attention figure) that help the model solve the task. 
	This example shows that regular indentation and spacing help \papertitle understand the form better just as they would help humans parse a form.
	The \textcolor{orange}{\textbf{orange}} boxed region in the heatmap also shows strong self-attention. We think that is due to \papertitle representing the blob of text as a single paragraph (in this case, as background text). Best viewed digitally and in color. }

	\label{fig:funsd_supplemental_atten_map}
\end{figure*}

\subsection{CORD Visualizations}
\papertitle matches the state-of-the-art performance of 96.33\% F1-score on CORD \cite{park2019cord} dataset (previous state-of-the-art model TILT-large consists of 780M parameters almost 4x the size of \papertitle). Please see Section 4.3 in the main paper.

In this sub-section we look at CORD \cite{park2019cord}  visualizations by \papertitle. We explicitly show hard-cases where \papertitle does well, see Figures \ref{fig:cord_supplemental_viz1}, \ref{fig:cord_supplemental_viz1_2},  \ref{fig:cord_supplemental_viz1_3}, \ref{fig:cord_supplemental_viz2_1}, \ref{fig:cord_supplemental_viz2_2}. In order to be transparent, we also show an error scenario in Figure \ref{fig:cord_supplemental_viz2_3}. Legend for the colors in images is, Menu items: \textcolor{red}{\textbf{Red}}, Total: \textcolor{blue}{\textbf{Blue}}, Sub-total (pre-tax): \textcolor{green}{\textbf{Green}}, Void-menu: Cyan color, Other: grey. 

%show the ground truth, predictions and visual attention weights for images from the CORD test set. Figures \ref{fig:cord_supplemental_viz2_1}, \ref{fig:cord_supplemental_viz2_2} show success cases and \ref{fig:cord_supplemental_viz2_3} shows a minor error case. 

\begin{figure*}
	\centering
	\subcaptionbox{Ground Truth (left) and \papertitle predictions (right)}[.63\linewidth][c]{%
	\includegraphics[width=\linewidth]{images/viz_receipt_00053}}\quad
	%\subcaptionbox{\papertitle multi-modal attention map}[.31\linewidth][c]{%
	%\includegraphics[width=\linewidth]{images/viz_attn_receipt_00053_attn.png}}\quad
	\caption{\textbf{\papertitle predictions on CORD}: For file receipt\_00053 (a) shows both ground-truth and predictions. \papertitle predicted correctly all the entity regions in the image. Best if viewed digitally and in color.}
	\label{fig:cord_supplemental_viz1}
\end{figure*}

%In (b) from the attention map, we can see that \papertitle learned to attend to regions in the image where text is present. Notice, it learned to ignore text in the header and blurred text.

\begin{figure*}
	\centering
	\subcaptionbox{Ground Truth (left) and \papertitle predictions (right)}[.63\linewidth][c]{%
	\includegraphics[width=\linewidth]{images/cord_supp_viz3/44_gt_pred.png}}\quad
	%\subcaptionbox{\papertitle multi-modal attention map}[.31\linewidth][c]{%
	%\includegraphics[width=\linewidth]{images/cord_supp_viz3/44_attn.png}}\quad
	\caption{\textbf{\papertitle predictions on CORD}: For file receipt\_00044. Best if viewed digitally and in color.}
	\label{fig:cord_supplemental_viz1_2}
\end{figure*}

\begin{figure*}
	\centering
	\subcaptionbox{Ground Truth (left) and \papertitle predictions (right)}[.63\linewidth][c]{%
	\includegraphics[width=\linewidth]{images/cord_supp_viz3/72_gt_pred.png}}\quad
	%\subcaptionbox{\papertitle multi-modal attention map}[.31\linewidth][c]{%
	%\includegraphics[width=\linewidth]{images/cord_supp_viz3/72_attn.png}}\quad
	\caption{\textbf{\papertitle predictions on CORD}: For file receipt\_00072. Best if viewed digitally and in color.}
	\label{fig:cord_supplemental_viz1_3}
\end{figure*}

\begin{figure*}
	\centering
    \subcaptionbox{Ground Truth}[.40\linewidth][c]{%
	\includegraphics[width=\linewidth]{images/cord_supp_viz2/04_gt.png}}\quad
	\subcaptionbox{\papertitle predictions}[.40\linewidth][c]{%
	\includegraphics[width=\linewidth]{images/cord_supp_viz2/04_pred.png}}\quad

	\caption{\textbf{\papertitle perfect predictions on CORD dataset}: Left image shows GT and right image is the prediction for file receipt\_00004 made by \papertitle which perfectly matches with the GT despite the presence of distortion and background text.} 

	\label{fig:cord_supplemental_viz2_1}
\end{figure*}

\begin{figure*}
	\centering
    \subcaptionbox{Ground Truth}[.40\linewidth][c]{%
	\includegraphics[width=\linewidth]{images/cord_supp_viz2/51_gt.png}}\quad
	\subcaptionbox{\papertitle predictions}[.40\linewidth][c]{%
	\includegraphics[width=\linewidth]{images/cord_supp_viz2/51_pred.png}}\quad

	\caption{\textbf{\papertitle perfect predictions on CORD dataset}: Left image shows GT and right image is the prediction for file receipt\_00051 made by \papertitle which perfectly matches with GT. Note that the faded out text which is hard to OCR is correctly classified due to multi-modal self-attention features.} 

	\label{fig:cord_supplemental_viz2_2}
\end{figure*}

\begin{figure*}
	\centering
    \subcaptionbox{Ground Truth}[.40\linewidth][c]{%
	\includegraphics[width=\linewidth]{images/cord_supp_viz2/85_gt.png}}\quad
	\subcaptionbox{\papertitle predictions}[.40\linewidth][c]{%
	\includegraphics[width=\linewidth]{images/cord_supp_viz2/85_pred.png}}\quad

	\caption{\textbf{\papertitle Partially correct predictions on CORD dataset}: Left image shows GT and right image is the prediction for file receipt\_00085 made by \papertitle with a misclassification of tokens of category SUBTOTAL with TOTAL items. This could be due to the rarity of SUBTOTAL tokens appearing below TOTAL tokens which \papertitle may not have encountered during training. } 

	\label{fig:cord_supplemental_viz2_3}
\end{figure*}
